# Supplementary material for: Development and Benchmarking of JANGOFETT: A Novel Geant4-Operated Fission Event Tracking Tool
Source: arXiv:2503.04791 source file (2025-06-09)
Supplement: Supplementary file 1 [file JANGOFETT_Supplemental_Material.pdf]

# Supplementary Material for The Development and Benchmarking of JANGOFETT: A Geant4-Based Fission Event Tracking Tool

Liam Walker[1], Jack Shire[1], Jacob Jaffe[1], Payton Sprando[1], Jack Olinger[1], and Alexander Chemey[1]

[1]Department of Nuclear Science and Engineering, Oregon State University, Corvallis, OR 97331, United States

## 1 Simulation Geometry

The design of the detector system used for analysis of JANGOFETT is illustrated in Fig S.1. A custom scattering chamber was centered in the simulation world, constructed of aluminum with a 50 $\mu$m sphere of polyethylene terephthalate (Mylar). Within the chamber are two 100 cm$^2$ silicon detectors of 300 micron thickness used for charged particle spectroscopy. These were placed on opposite sides at an offset of 4 cm from the center of the detector to the source. At the center of the chamber, two fission fragments were emitted from the origin in sequential Geant4 events.

The detector system simulated in Geant4 included 21 high-purity germanium (HPGe) detectors arranged equidistantly around the primary fission product (PFP) source location at a distance of 20 cm. Detectors were placed orthogonal to each face of a truncated cuboctahedron scattering chamber comprised of 8 triangular surfaces and 18 square surfaces. Two square face detectors openings were removed for simulated up- and downstream beam port locations, and 3 square faces in the lower hemisphere were removed due to constraints with the real-world floor (not modeled).

Each HPGe was surrounded by an annular bismuth germanium oxide (BGO) active veto detector for Compton suppression. Simulated HPGe detector geometries included genericized planar, coaxial, and clover style detectors, ranging from 15

## 2 Coincidence Timing

The identification of the $\gamma$-coincidence timing window was performed by analyzing the timing between fissions and coincident prompt $\gamma$ pulses in Fig S.2. First, the average time between coincident fragment pairs (PFP) triggers in the silicon detectors was determined to be less than 5 ns. Then, a secondary timing window was defined around this average to effectively capture the majority of coincident prompt $\gamma$-rays, as illustrated in Fig. S.2. A broad coincidence window of -30 ns to 20 ns was selected for silicon-HPGe coincidences, where t = 0 is chosen to be the average silicon detector trigger time for valid

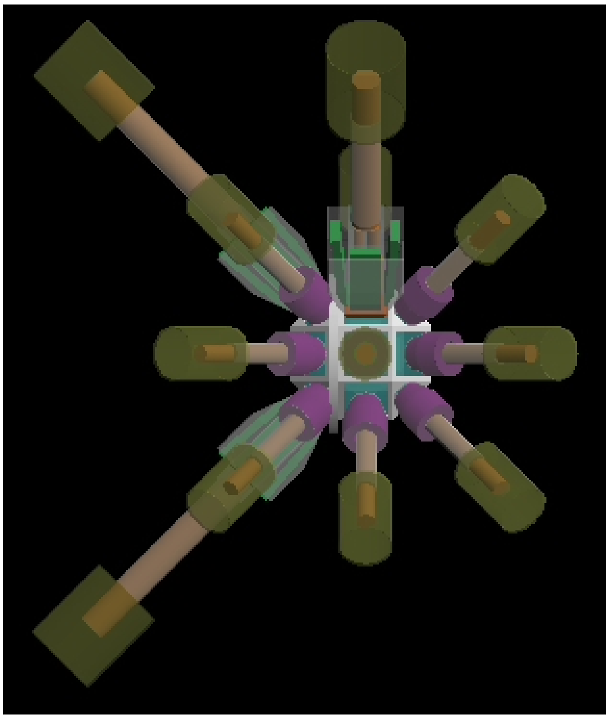

Figure S.1: Ray traced render of the Geant4 world geometry. All detectors are placed such that the crystals are 20 cm from the origin. Color code: Teal is the scattering chamber Mylar window, silver is the scattering chamber structure, light green are BGO crystals for the clover detectors, purple are BGO detector housings for the planar and coaxial detectors, brown is an aluminum “cold finger,” and off-yellow is the dewar for the detectors. HPGe crystals and silicon detectors are not shown in this image as they are internal to the Mylar window.

silicon-silicon coincidence events with deposited energy greater than 20 MeV. With this timing established, the coincidence information was extracted as correlated events, enabling straightforward filtering between light and heavy fragment pairs, as well as PFP-$\gamma$ coincidences.

# 3 Total Kinetic Energy

Total kinetic energy was calculated by summing the energy depositions within the silicon detectors that occurred within 20 ns of each other. Due to the nature of beam-line experiments, there is a chance that 3 or 4 fragments may hit the detector in this time creating a false coincidence. It was important that this simulation be able to demonstrate the ability to reproduce this effect to replicate the noise expected in real life experiments. This is shown clearly in Fig S.3, where the false coincidences extend from 230 to 400 MeV of ”TKE”, although input TKE never exceeded $\sim$225 MeV in the CGMF simulation. Note that the 4-fragment cluster is larger than the 3-fragment cluster. This is due to the geometry of the simulation - PFP are emitted at almost 180° in the lab frame, with small deviations for momentum transfer from emitted neutrons, so if one fragment is detected, its complement is also likely to be detected. These multi-hit events occurred a total of 793 times of the $7.19924 \times 10^7$ fission fragment silicon detector pulses recorded, 0.0011

A potential source of error would be a systematic distortion or bias in Geant4 or

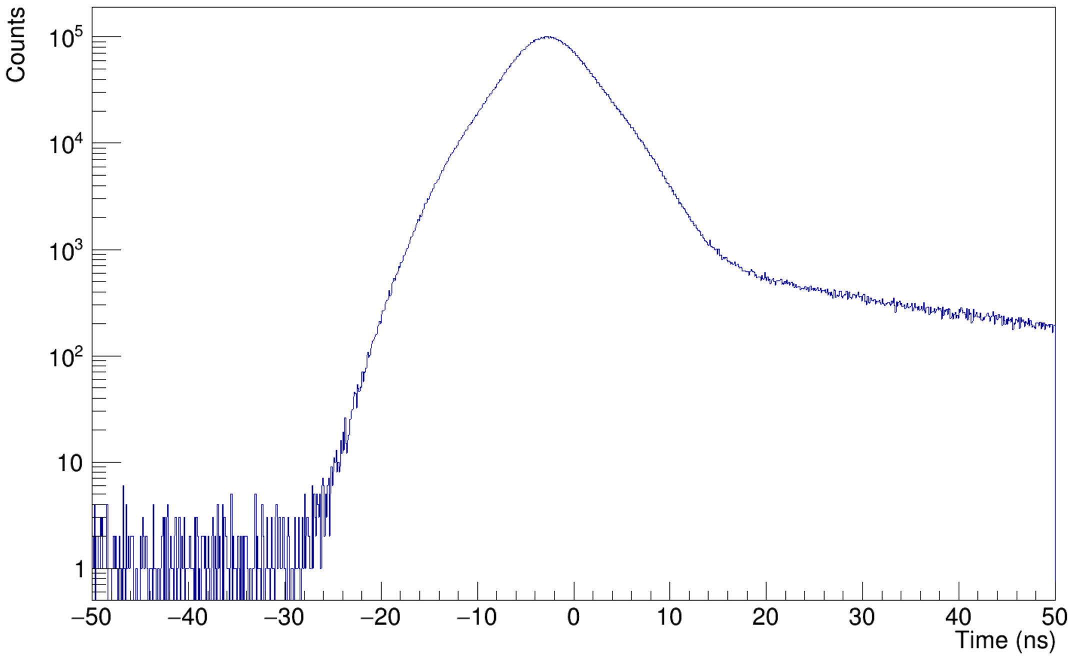


Figure S.2: Coincidences for $\gamma$ pulses near the averaged time for a coincident pair of PFP pulses from -30 ns to +20 ns vs the average silicon detector trigger time. The main peak is centered around -3.6 ns, as primary fission products (PFPs) tend to trigger ∼3.6 ns after photon events in HPGe detectors.

our analysis code, one that did not match the inputs from CGMF. This is most easily checked by comparing TKE values from CGMF and the output from Geant4, both in mean TKE and in the distribution of TKE. Shown in Fig S.4 are the mean TKE for (post Geant4- simulation) Geant4 and CGMF (inputs for the Geant4 simulation). These data are within reasonable agreement. The distribution from Geant4 is slightly flatter than the inputs, which is to be expected given the blurring applied to the detectors, and is shifted very modestly (ca. 4.1 keV) to the low-energy side, approximately one standard error of the mean, due to secondary particles and X-rays emitted from the surface of the silicon detectors. Standard deviations of the fit ($\sigma$) are consistent as well, only differing in the Geant4-simulated distribution is 4.5 keV broader due to the Gaussian blurring.

# 4 Additional Gated Fragments

In addition to $^{144}$Ba, $^{141}$Cs, $^{149}$Nd, and $^{150}$Ce were also gated on using the methods described in section 3.3 of the paper. All of the $\gamma$-$\gamma$-$\gamma$ histograms for the respective fragments are provided below, as are the $\gamma$ gates, selected from the Brookhaven NNDC data for excited states of each isotope, utilizing NuDat3 data [National Nuclear Data Center(*accessed 2025*)].

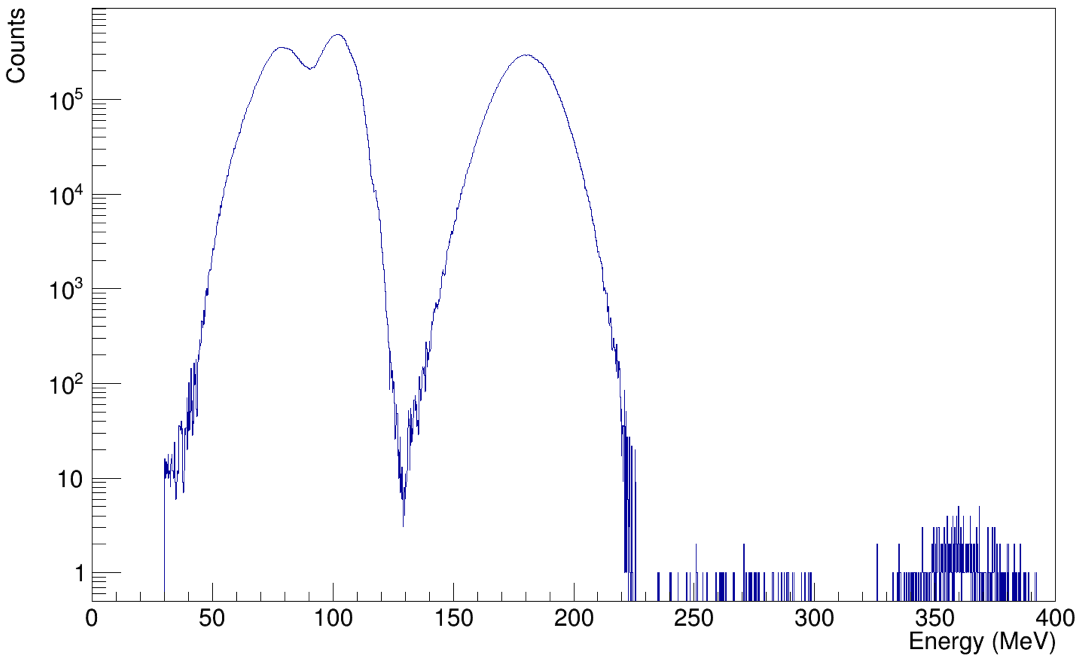


Figure S.3: Charged particle spectra from DSSD pulses. Shown here is the TKE and KE on the same figure (see text for fit information). Note that there are a small number of events beyond the edge of the actual coincident TKE events (beyond 230 MeV) representing false coincidences. The first small cluster from about 230-300 MeV are the 3 fragment coincidences, and the 320-400 MeV cluster is the double pair (4 fragment) coincidences.

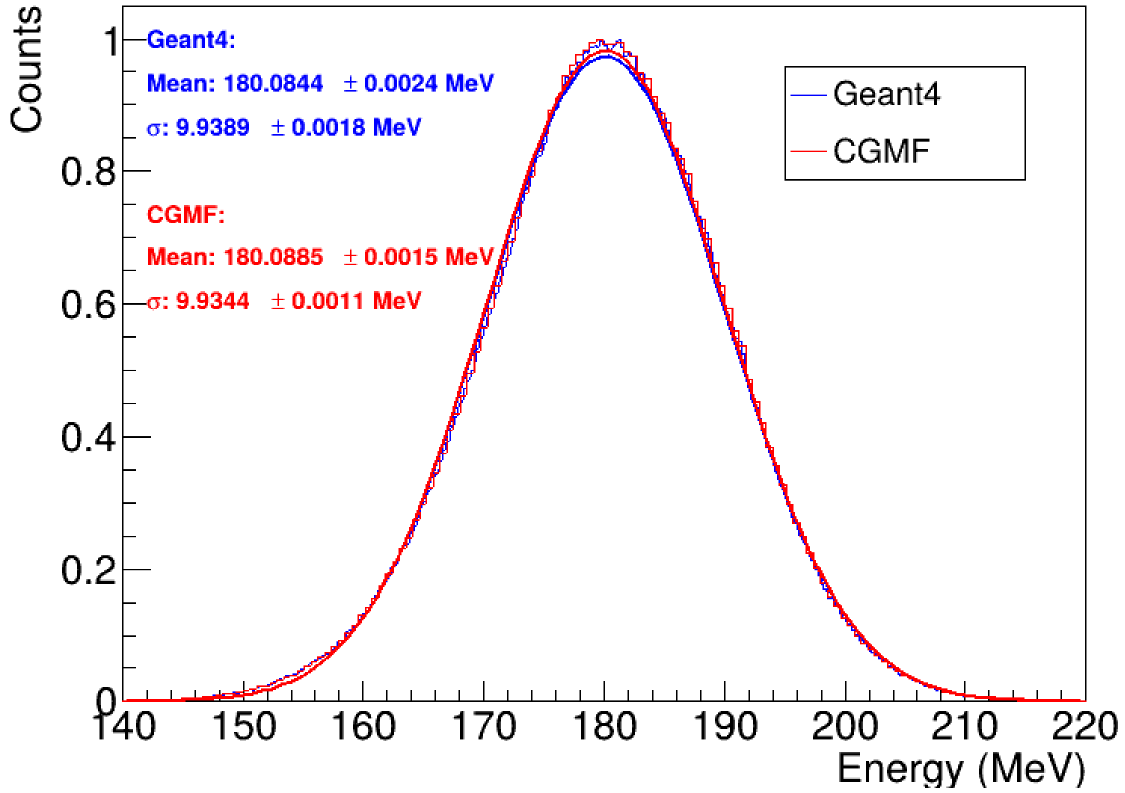


Figure S.4: Overlayed and normalized TKE for the data, with Gaussian fits, before and after CGMF inputs are simulated in Geant4. Distributions are modest and differences are explicable, see text in Supplementary Material.

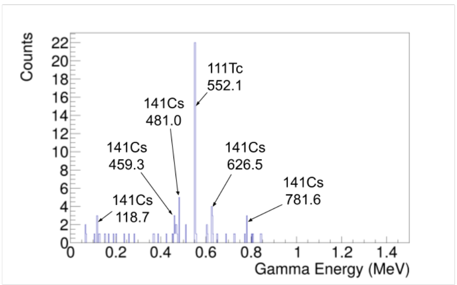


(a) 0n

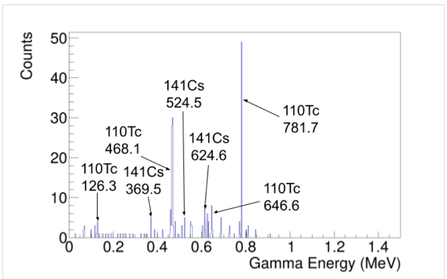


(b) 1n

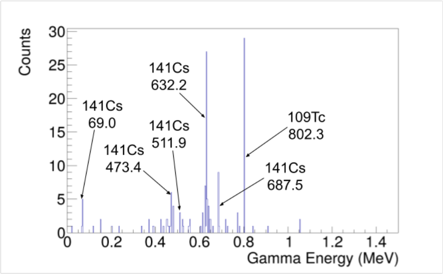


(c) 2n

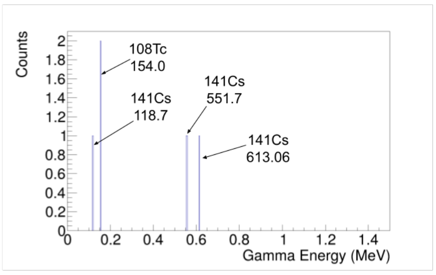


(d) 3n

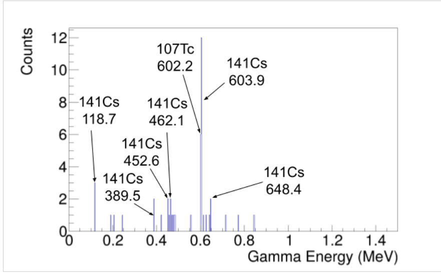


(e) 4n

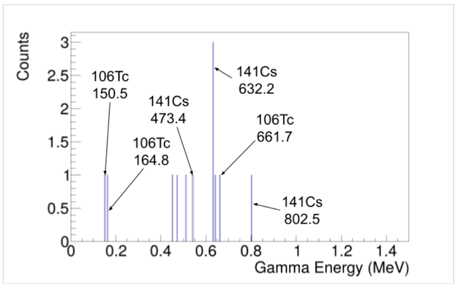


(f) 5n

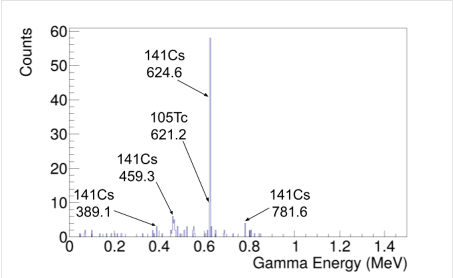


(g) 6n

Figure S.5: $\gamma$ energy spectra when at least two coincident $\gamma$ from $^{141}$Cs and at least one $\gamma$ from the correlated light fragment (i.e. $^{252}$Cf$\rightarrow$ $^{144}$Ba+$^{A}$Mo+$X$n), for x between 0 and 6 for (a) through (g). Energy labels on the figure are given in keV with the respective PFP label.

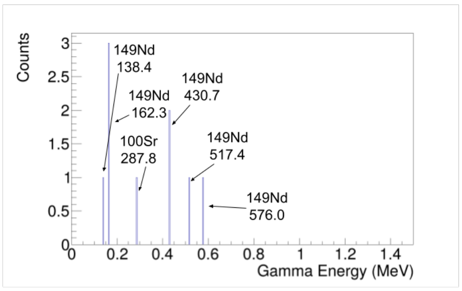


(a) 3n

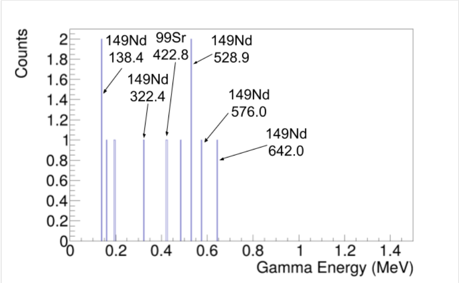


(b) 4n

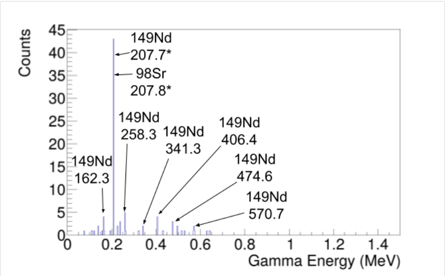


(c) 5n

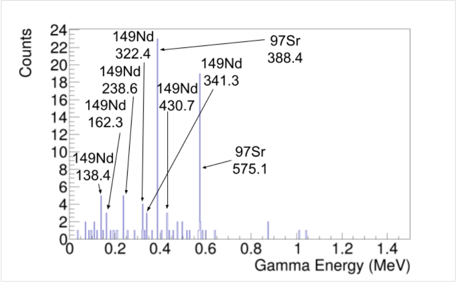


(d) 6n

Figure S.6: $\gamma$ energy spectra when at least two coincident $\gamma$ from $^{149}$Nd and at least one $\gamma$ from the correlated light fragment (i.e. $^{252}$Cf$\rightarrow$ $^{144}$Ba+$^{A}$Mo+$X$n), for x between 3 and 6 for (a) through (d). Energy labels on the figure are given in keV with the respective PFP label. Note that "*" denotes an energy that may appear from either the light or heavy fragment. The "*" energies were not selected for making gates on these coincidences.

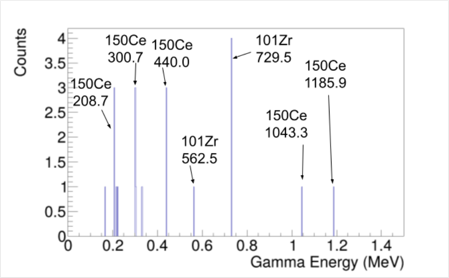


(a) 1n

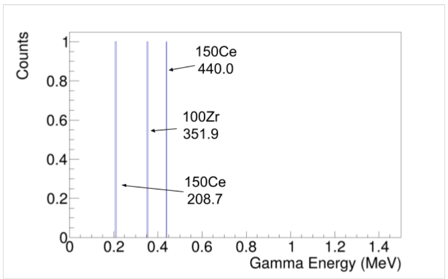


(b) 2n

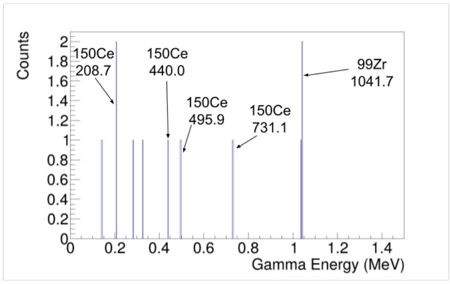


(c) 3n

Figure S.7: $\gamma$ energy spectra when at least two coincident $\gamma$ from $^{150}$Ce and at least one $\gamma$ from the correlated light fragment (i.e. $^{252}$Cf$\rightarrow$ $^{144}$Ba+$^{A}$Mo+$X$n), for x between 1 and 3 for (a) through (c). Energy labels on the figure are given in keV with the respective PFP label.

Table 1: $^{144}$Ba and light fragment compliment $\gamma$ gates

| Isotope | Gamma Energy Gates (keV) |
|---|---|
| $^{144}$Ba | 199.326, 330.88, 559.57, 758.96, 638.99, 431.3, 820.71, 508.7, 1116.42, 393.7, 1078.63, 1089.08, 1025.73, 1664.98, 1350.8, 952.8, 1029.8, 573.5, 1197.7, 348.06, 506.1, 892, 2176, 504.7, 622.8, 584.6, 624.6, 653.7, 655.3, 670.8, 723.1, 785.5 |
| $^{108}$Mo | 192.7, 370.9, 590.1, 392.4, 414.6, 527, 449.2, 529.5, 915.8, 662.1, 662.3 |
| $^{107}$Mo | 65.4, 66, 152.1, 165.4, 154.3, 253.7, 341, 110.2, 326.3, 414.5, 123.4, 410.8, 478.8, 256.1, 379.5, 405.9, 551.2, 556, 555, 602.8, 557.5, 620.7, 679, 687.8, 709, 720, 698.7, 750.5 |
| $^{106}$Mo | 171.548, 350.69, 538.88, 174.6, 511.2, 896.23, 1108.3, 724.5 |
| $^{105}$Mo | 94.8, 137.9, 246.9, 309.9, 85.3, 253.7, 144.8, 283, 150, 369.3, 159.029, 514, 192.5, 245.8, 390.8, 415.9, 553.8, 185.6, 266.6, 369.9, 418.3, 775.6, 356.2, 457.2, 686.4, 831.4, 415.2, 468.4, 552.6, 526.2, 679, 924.8, 557.1, 484, 528.5, 664.1, 588.5, 540, 600.2, 736.5, 632.7, 578.4, 704.8, 705.8, 651.3, 694, 572.1, 642.8, 859.8, 677.2, 658.8, 708.2, 647.1 |
| $^{104}$Mo | 192.2, 368.4, 620.2, 812.4, 693.9, 836.3, 519.2, 1022.7, 1083, 1468.4, 914.9, 1352.3, 771.3, 1414.6, 1050, 1063.9, 641.7, 509.8, 644.2, 1229.6, 609.3, 796.1, 1322.5, 561.2, 477.5, 868.6, 150.7, 387.8, 628.6, 1225, 2124.8, 601.7, 289.3, 548.6, 184.3, 571.6, 733.6 |
| $^{103}$Mo | 102.561, 138.5, 346.5, 251.18, 456.2, 124.9, 143.3, 144.5, 526.1, 397, 641.1, 687.5, 236.8, 590.4, 746.3, 372.3, 363.1, 468.3, 967.1, 572.2, 519.2, 729.7, 1083, 547, 575.7, 706.8, 738, 755.5 |

Table 2: $^{141}$Cs and light fragment compliment $\gamma$ gates

| Isotope | Gamma Energy Gates (keV) |
|---|---|
| $^{141}$Cs | 69.05, 47.78, 118.705, 100.721, 369.5, 389.11, 467.81, 423.89, 556.8, 462.1, 613.06, 842.7, 772.9, 473.4, 481.0, 909.23, 1051.96, 641.19, 551.7, 632.2, 626.5, 687.5, 459.3, 726.5, 781.6, 810.3, 452.6, 511.9, 603.9, 624.6, 648.4, 802.5, 524.5 |
| $^{111}$Tc | 131.8, 284.2, 375.8, 410.6, 312.7,419.5,552.1, 606.7, 660.2, 723.8,544.5 |
| $^{110}$Tc | 126.3, 178.3, 357.1, 487.7, 468.1, 646.6, 616.1, 781.7,745.8 |
| $^{109}$Tc | 137.0, 298.0, 437.5, 440.3, 587.6, 564.7, 719.7, 802.3, 685.5, 633.2, 761.0,426.2, 332.4, 629.9, 671.0 |
| 20 $^{108}$Tc | 86.4, 106.2, 268.3, 240.5, 154.0, 224.1, 218.5, 682.7, 601.0, 312.7 |
| $^{107}$Tc | 602.28, 415.4, 788.74, 733.46, 509.26, 548.23, 703.16, 482.55 |
| $^{106}$Tc | 164.8, 661.7, 150.5, 254.5, 272.8, 717.0, 158.4, 542.5 |
| $^{105}$Tc | 471.2, 623.43, 744.95, 784.4, 314.34, 427.16, 495.11, 503.27, 279.14, 364.3, 706.25, 625.18, 435.7, 621.20, 732.24, 187.7, 207.8 |

Table 3: $^{149}$Nd and light fragment compliment $\gamma$ gates

| Isotope | Gamma Energy Gates (keV) |
|---|---|
| $^{149}$Nd | 108.52, 138.447, 165.087, 112.185, 258.327, 162.338, 120.395, 207.71, 321.124, 332.944, 69.5, 365.953, 238.638, 341.31, 459.52, 474.57, 197.194, 517.44, 227.481, 406.4, 322.4, 494.9, 389, 570.72, 576.03, 528.91, 642.03, 430.76, 874.11 |
| $^{100}$Sr | 129.2, 287.8, 434.8, 808.6, 1257.1, 1186.2, 1197.4, 1285.5, 566.3, 1289.5, 1371.3, 1392.6, 1143.4, 1201.7, 1231, 1328.7, 161.8, 1539.4, 1827.8, 194.4, 1926.8, 689.9, 2115.6, 2211.6, 2148.4, 864 |
| $^{99}$Sr | 90.8, 125.2, 161, 422.8, 318, 192, 304.4, 307, 763.8, 854.7, 646.2, 903.8, 846.8, 1071.6, 683.8, 936, 965.1, 1104.9, 1149.8, 1112, 1291.8, 1211.1, 1664, 1578.5, 1668.6, 1972, 2230 |
| $^{98}$Sr | 144.7, 71, 289.4, 433.3, 655.8, 1079.7, 566.3, 1323.9, 1455.9, 810.4, 1600.6, 1693.2, 1777.7, 1819.5, 140.6, 689.5, 1979.6, 1719.5, 1772, 630.7, 1359.8, 2092.9, 2144.5, 2171.5, 1925.5, 207.8, 1564.7 |
| $^{97}$Sr | 167.1, 141, 144.9, 355.3, 585.2, 600.5, 644.6, 520, 69.1, 588.3, 768.7, 57.7, 237.3, 522.7, 749.4, 232.7, 985.3, 223.8, 205.9, 95.1, 375.5, 283, 735.6, 396, 687.7, 388.4, 442.9, 1507.3, 509.7, 561, 522.8, 575.1, 638 |

Table 4: $^{150}$Ce and light fragment compliment $\gamma$ gates

| Isotope | Gamma Energy Gates (keV) |
|---|---|
| $^{150}$Ce | 97, 208.7, 300.7, 376.2, 779.2, 440, 890.8, 1012.4, 1097.5, 750.1, 1153.7, 1178, 1185.9, 495.9, 993.7, 1043.3, 325, 731, 303, 1353.2, 945.9, 232.5, 546.5 |
| $^{101}$Zr | 216.68, 133.67, 104.43, 309.98, 146.64, 378.8, 152.1, 575.47, 527.32, 759.45, 688.4, 487.44, 729.57, 746.7, 450.2, 249.8, 648.59, 670.67, 710.2, 727.3, 940.2, 428.1, 510, 222.6, 1119, 1297.89, 1300.26, 259.8, 562.5, 578.3, 904, 1297.7, 569, 295.6, 629.1, 777.6, 2023.06, 331.3, 1984.7, 696.7, 712.5, 365, 738.6 |
| $^{100}$Zr | 212.61, 118.63, 351.966, 616.67, 666, 1196.09, 1082.33, 850.24, 1228.99, 625.55, 1595.16, 1291.6, 1346.6, 1059.51, 1438.6, 1191.6, 1566.05, 244.8, 810.1, 1655.8, 1680, 845.2, 1254.2, 1471, 739, 1405.6, 1409.7, 219.9, 1434.7 |
| $^{99}$Zr | 121.7, 130.2, 575.7, 614.2, 536.2, 53.3, 426.7, 724.4, 639.9, 782.3, 143, 192.7, 600.1, 189.3, 885.2, 706.7, 1005.5, 929.5, 1064.7, 407.7, 957.2, 268.7, 570.6, 392.5, 572.3, 415, 1003.8, 619.3, 411.6, 472.8, 476.2, 1311.1, 830.8, 251.1, 519.8, 1548.5, 1041.7, 954.4, 283.3, 566, 1834.5, 604, 570, 1074.6, 1957.4, 313.8, 624.2, 1572.7, 1742.7, 1790.6 |

## References

[National Nuclear Data Center(*accessed 2025*)] National Nuclear Data Center, *accessed 2025*. Information extracted from the nudat database. URL: `https://www.nndc.bnl.gov/nudat/`. available online at `https://www.nndc.bnl.gov/nudat/`.
